# Supplementary material for: The Grammar-Learning Trajectories of Neural Language Models
Source: arXiv:2109.06096 source file (2022-04-06)
Supplement: Supplementary file 1 [file appendix.tex]

% This must be in the first 5 lines to tell arXiv to use pdfLaTeX, which is strongly recommended.
\pdfoutput=1
% In particular, the hyperref package requires pdfLaTeX in order to break URLs across lines.

\documentclass[11pt]{article}

\usepackage{xr-hyper}

\usepackage[review]{emnlp2021}
\usepackage{times}
\usepackage{latexsym}
\usepackage{graphicx}
\graphicspath{{graphs/}}
\graphicspath{{graphs/}}

\usepackage{placeins}

 %\newcommand{\oa}[1]{}

% This is not strictly necessary, and may be commented out,
% but it will improve the layout of the manuscript,
% and will typically save some space.
\usepackage{microtype}

% for subfigures
\usepackage{caption}
\usepackage{subcaption}
\usepackage{xcolor}

%\aclfinalcopy % Uncomment this line for the final submission
%\def\aclpaperid{***} %  Enter the acl Paper ID here

%\setlength\titlebox{5cm}
% You can expand the titlebox if you need extra space
% to show all the authors. Please do not make the titlebox
% smaller than 5cm (the original size); we will check this
% in the camera-ready version and ask you to change it back.

\title{Language Generation is Learnt in this Order.}
\appendix
\author{First Author \\
  Affiliation / Address line 1 \\
  Affiliation / Address line 2 \\
  Affiliation / Address line 3 \\
  \texttt{email@domain} \\\And
  Second Author \\
  Affiliation / Address line 1 \\
  Affiliation / Address line 2 \\
  Affiliation / Address line 3 \\
  \texttt{email@domain} \\}

\date{}

\begin{document}
\maketitle

\appendix
\input{paper/appendix_content}

\bibliography{acl2020}
\bibliographystyle{acl_natbib}
\end{document}
